# Supplementary material for: Astability versus Bistability in van der Waals Tunnel Diode for Voltage Controlled Oscillator and Memory Applications
Source: arXiv:2010.13828 source file (2020-10-26)
Supplement: Supplementary file 1 [file supporting_info.pdf]

# Astability *versus* Bistability in van der Waals Tunnel Diode for Voltage Controlled Oscillator and Memory Applications

Nithin Abraham,† Krishna Murali,† Kenji Watanabe,‡ Takashi Taniguchi,¶ and Kausik Majumdar*,†

†*Department of Electrical Communication Engineering, Indian Institute of Science, Bangalore 560012, India*

‡*Research Center for Functional Materials, National Institute for Materials Science, 1-1 Namiki, Tsukuba 305-0044, Japan*

¶*International Center for Materials Nanoarchitectonics, National Institute for Materials Science, 1-1 Namiki, Tsukuba 305-0044, Japan*

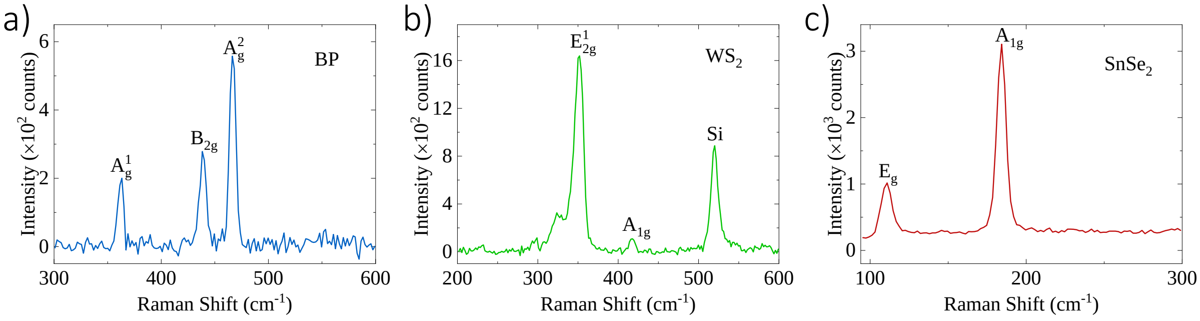


Supplementary Figure 1: **Raman characterization for different flakes:** Raman spectra of **a)** BP, **b)** $WS_2$, **c)** $SnSe_2$, collected with 532 nm excitation.

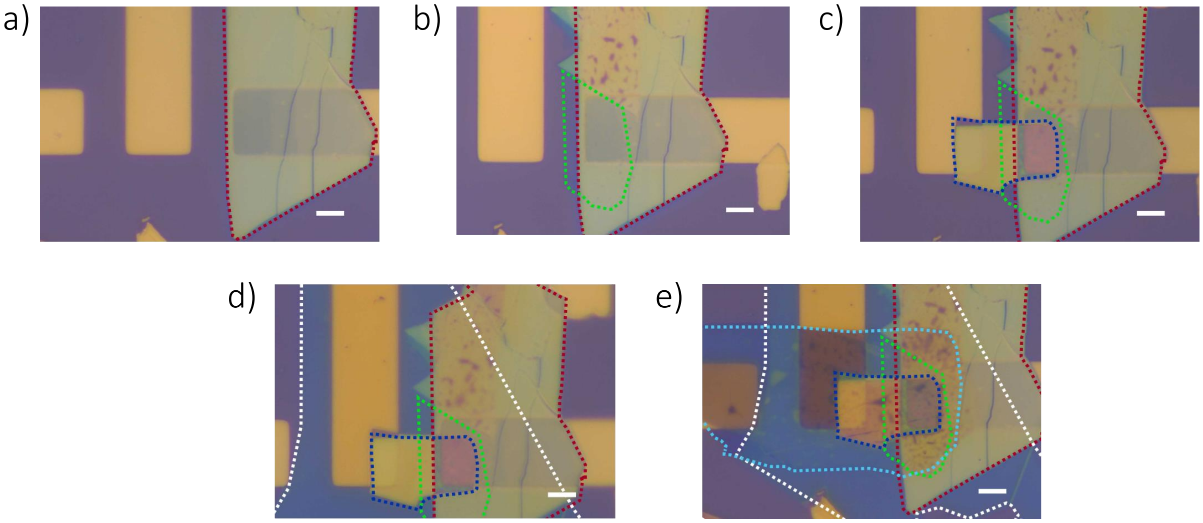


Supplementary Figure 2: **Fabrication steps for tunnel diode:** **a)** Transfer of $SnSe_2$ (Red dotted trace). **b)** Transfer of 1L-$WS_2$ with precise alignment (Green dotted trace). **c)** Transfer of few layer BP (Blue dotted trace). **d)** Encapsulation with hBN (White dotted trace). **e)** Transfer of graphene for gate contact (Cyan dotted trace). Scale bar is 5 $\mu m$.

Supplementary Table 1: Summary of tunnel diode performance from multiple samples using BP/1L-$WS_2$/$SnSe_2$ heterojunction

| Device | Barrier | $J_p$ ($A/cm^2$) | $J_v$ ($A/cm^2$) | PVCR | Temperature (K) | Annealing |
|---|---|---|---|---|---|---|
| D1 | 1L $WS_2$ | 2.68 | 0.74 | 3.60 | 300 | After $WS_2$ |
| | | 1.74 | 0.38 | 4.58 | 7 | |
| D2 | 1L $WS_2$ | 18.07 | 5.56 | 3.25 | 300 | After $WS_2$ |
| D3 | 1L $WS_2$ | 0.08 | 0.03 | 3.00 | 300 | Not annealed |
| | | 14.66 | 6.67 | 2.20 | | After BP (Vacuum) |
| D4 | 1L $WS_2$ | 10.63 | 6.24 | 1.70 | 300 | After $WS_2$ |
| D5 | 1L $WS_2$ | 4.56 | 3.24 | 1.40 | 300 | After BP |
| D6 | 1L $WS_2$ | 2.91 | 0.88 | 3.32 | 300 | After $WS_2$ |
| D7 | 1L $WS_2$ | 0.17 | 0.05 | 3.60 | 300 | Not annealed |
| | | 0.25 | 0.05 | 4.82 | 205 | |

Supplementary Table 2: Role of barrier layer on tunnel diode performance

| Device | Barrier | $J_p$ ($A/cm^2$) | $J_v$ ($A/cm^2$) | PVCR | Temperature (K) | Annealing |
|---|---|---|---|---|---|---|
| D8 | None | 21.90 (@$V_D$=0.5 V) | | No NDR | 300 | Not annealed |
| D1 | 1L $WS_2$ | 2.68 | 0.74 | 3.60 | 300 | After $WS_2$ |
| D9 | 2L $WS_2$ | 0.06 | 0.03 | 2.00 | 300 | Not annealed |
| D10 | 1L $MoS_2$ | 9.50 | 8.56 | 1.11 | 300 | After $MoS_2$ |

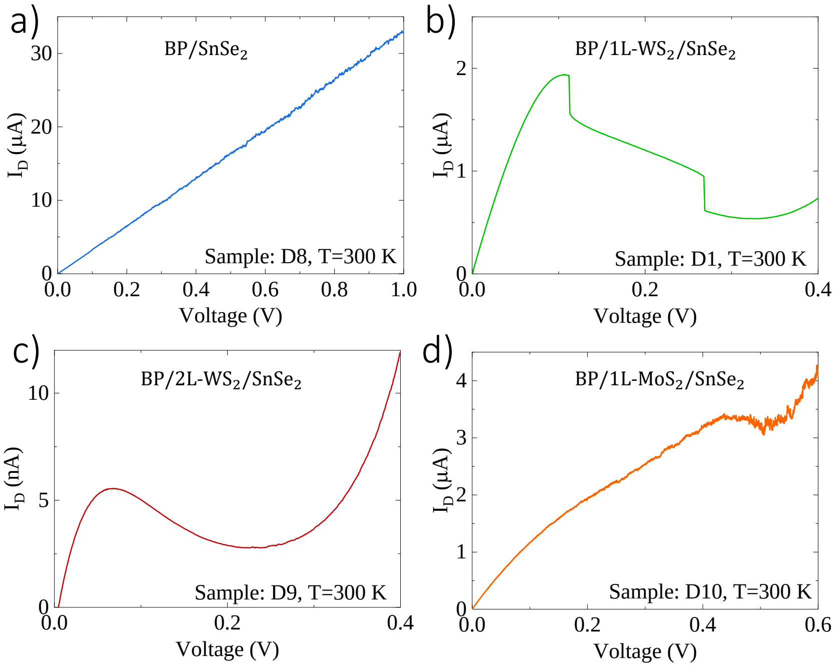


Supplementary Figure 3: **Different choice of barrier layers: a)** $I_D - V_D$ curves from samples with **a)** no barrier showing a large and linear tunnelling current, **b)** 1L-WS$_2$ barrier with a large PVCR, **c)** 2L-WS$_2$ barrier exhibiting moderate PVCR, but with a considerably lower $I_P$ and **d)** 1L-MoS$_2$ barrier with a degraded PVCR.

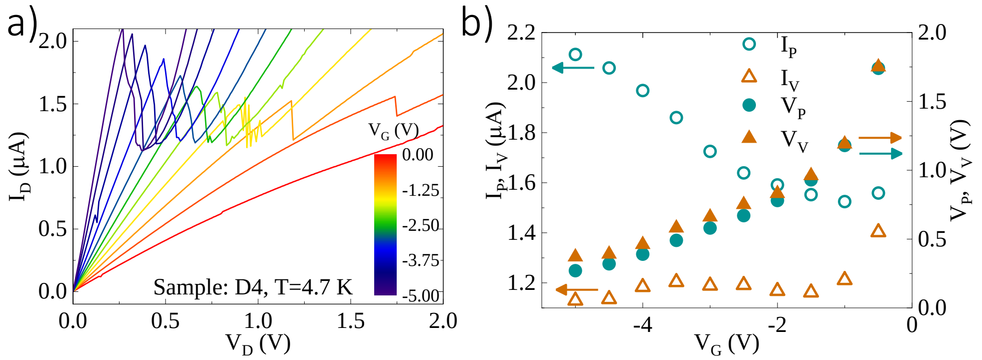


Supplementary Figure 4: **Gate modulation of output characteristics: a)** $I_D - V_D$ curves from sample D4 employing a thin BP layer at 4.7 K as a function of gate bias ranging from 0 to $-5$ V. **b)** Left axis: Modulation of peak (empty teal circle markers) and valley (empty orange triangle markers) currents with gate bias. $I_P$ increases with an increase in the negative $V_G$ suggesting an increase in the $p$-type doping in BP. Right: Peak (solid teal circle markers) and valley (solid orange triangle markers) positions also exhibit a shift to higher voltages in accordance with the increasing drop across $R_s$ as $V_G$ approaches lesser negative values.

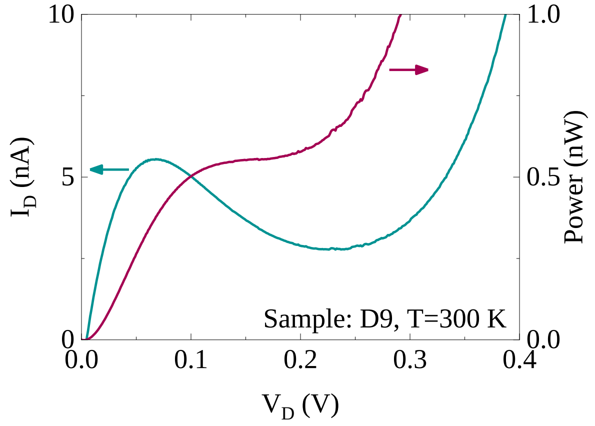


Supplementary Figure 5: **Absence of oscillation for 2L-$WS_2$ barrier:** Left axis: $I_D - V_D$ characteristics from sample D9 employing 2L-$WS_2$ as the tunnel barrier at 300 K showing no oscillations. Right: Power delivered corresponding to each applied $V_D$. Absence of multi-valued voltage at a given power further supports the disappearance of oscillations as we move to 2L-$WS_2$ barrier layer from 1L-$WS_2$.

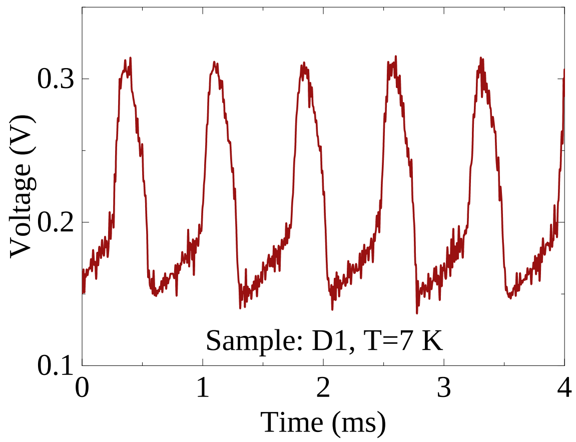


Supplementary Figure 6: **Astable operation mode:** Temporal response from D1 at 7 K exhibiting oscillations when biased in the NDR regime.
